# Supplementary material for: Assessment of the accuracy of coupled cluster perturbation theory for open-shell systems. I. Triples expansions
Source: arXiv:1512.02846 ancillary file (2016-02-19)
Supplement: Supplementary file 1 [file si.pdf]

# Supporting information for: Assessment of the accuracy of coupled cluster perturbation theory for open-shell systems. I. Triples expansions

Janus J. Eriksen,*,† Devin Matthews,‡ Poul Jørgensen,† and Jürgen Gauss¶

*qLEAP Center for Theoretical Chemistry, Department of Chemistry, Aarhus University, DK-8000 Aarhus C, Denmark, The Institute for Computational Engineering and Sciences, The University of Texas at Austin, Austin, Texas 78712, United States, and Institut für Physikalische Chemie, Johannes Gutenberg-Universität Mainz, D-55128 Mainz, Germany*

E-mail: janusje@chem.au.dk

*To whom correspondence should be addressed
†Aarhus University
‡The University of Texas at Austin
¶Johannes Gutenberg-Universität Mainz

In the following, results for the recovery of the CCSDT–CCSD (and CCSDTQ–CCSDT) correlation energy differences are presented in percentage points with respect to 100% for brevity. Results are reported for mean recoveries ($\Delta$) and mean deviations ($\delta$) as well as standard deviations around the means ($\Delta_{\text{std}}$ and $\delta_{\text{std}}$, respectively).

In all tables, VDZ and VTZ refer to the cc-pVDZ and cc-pVTZ basis sets, respectively, and we note that the frozen-core approximation has been invoked for all the calculations reported herein.

Table S1: Recoveries of CCSDT/CCSD correlation energy differences in percent (%) for an RHF reference.

| Molecule | CCSD(T) | | CCSD(T–2) | | CCSD(T–3) | | CCSD(T–4) | | CCSD(T–5) | | CCSD(T–6) | |
|---|---|---|---|---|---|---|---|---|---|---|---|---|
| | VDZ | VTZ | VDZ | VTZ | VDZ | VTZ | VDZ | VTZ | VDZ | VTZ | VDZ | VTZ |
| $C_2H_2$ | -3.44 | -0.32 | -15.08 | -11.42 | -7.63 | -8.22 | -1.32 | -0.45 | -0.93 | -1.15 | -0.22 | 0.01 |
| $C_2H_4$ | -6.06 | -2.68 | -16.65 | -12.72 | -7.41 | -7.68 | -1.99 | -1.24 | -1.05 | -1.08 | -0.43 | -0.26 |
| $CH_2$ ($^1A_1$) | -19.90 | -14.44 | -27.31 | -21.70 | -12.48 | -11.03 | -6.88 | -5.61 | -4.57 | -3.77 | -3.35 | -2.72 |
| $CH_2O$ | -4.50 | -1.01 | -13.66 | -10.67 | -8.35 | -8.12 | -1.09 | -0.44 | -1.74 | -1.62 | 0.04 | 0.18 |
| CO | -4.10 | -0.80 | -12.22 | -10.18 | -10.55 | -9.77 | -0.28 | 0.18 | -2.83 | -2.50 | 0.70 | 0.74 |
| $CO_2$ | -1.34 | 0.74 | -11.16 | -9.45 | -11.90 | -10.31 | 0.76 | 0.95 | -3.72 | -3.07 | 1.29 | 1.23 |
| $F_2$ | -2.91 | 0.04 | -15.12 | -11.33 | -7.63 | -7.37 | -2.11 | -1.10 | -1.47 | -1.32 | -0.59 | -0.29 |
| $H_2O$ | -5.07 | -0.99 | -12.63 | -9.39 | -4.82 | -5.32 | -0.97 | -0.51 | -0.45 | -0.48 | -0.12 | -0.05 |
| $H_2O_2$ | -2.97 | 0.15 | -13.82 | -10.41 | -6.62 | -6.74 | -1.56 | -0.74 | -0.99 | -0.94 | -0.37 | -0.15 |
| HCN | -1.67 | 0.87 | -13.50 | -10.45 | -7.68 | -8.26 | -1.02 | -0.18 | -1.06 | -1.31 | -0.16 | 0.08 |
| HF | -4.45 | -0.47 | -9.32 | -7.94 | -4.12 | -4.77 | -0.36 | -0.22 | -0.46 | -0.47 | -0.02 | 0.03 |
| HNO | -2.57 | 0.16 | -14.27 | -11.11 | -8.54 | -8.52 | -1.88 | -0.94 | -1.98 | -1.89 | -0.61 | -0.27 |
| HOF | -3.14 | -0.15 | -14.00 | -10.65 | -7.38 | -7.23 | -1.59 | -0.75 | -1.43 | -1.29 | -0.33 | -0.07 |
| $N_2$ | -0.63 | 1.54 | -12.57 | -9.72 | -7.37 | -7.89 | -0.97 | -0.12 | -1.03 | -1.24 | -0.19 | 0.06 |
| $N_2H_2$ | -2.42 | 0.19 | -14.46 | -11.14 | -7.41 | -7.79 | -1.64 | -0.83 | -1.15 | -1.24 | -0.41 | -0.18 |
| $NH_3$ | -6.62 | -2.70 | -14.59 | -10.82 | -5.12 | -5.66 | -1.19 | -0.76 | -0.45 | -0.51 | -0.14 | -0.08 |
| $O_3$ | -0.39 | 1.53 | -17.99 | -14.27 | -16.21 | -14.12 | -2.04 | -0.37 | -6.51 | -5.80 | 0.39 | 1.20 |
| $\Delta$ | -4.25 | -1.08 | -14.61 | -11.37 | -8.31 | -8.16 | -1.54 | -0.77 | -1.87 | -1.75 | -0.27 | -0.03 |
| $\Delta_{std}$ | 4.40 | 3.64 | 3.83 | 3.00 | 3.01 | 2.25 | 1.56 | 1.35 | 1.66 | 1.37 | 0.93 | 0.84 |

Table S2: Recoveries of CCSDT/CCSD correlation energy differences in percent (%) for a UHF reference.

| Molecule | CCSD(T) | | CCSD(T–2) | | CCSD(T–3) | | CCSD(T–4) | | CCSD(T–5) | | CCSD(T–6) | |
|---|---|---|---|---|---|---|---|---|---|---|---|---|
| | VDZ | VTZ | VDZ | VTZ | VDZ | VTZ | VDZ | VTZ | VDZ | VTZ | VDZ | VTZ |
| C | -25.14 | -18.53 | -29.04 | -22.75 | -10.05 | -8.24 | -3.85 | -3.15 | -1.60 | -1.31 | -0.71 | -0.58 |
| CCH | -14.09 | -8.86 | -22.24 | -17.23 | -11.01 | -10.49 | -4.64 | -3.34 | -3.03 | -2.64 | -2.01 | -1.49 |
| CF | -8.63 | -4.27 | -12.76 | -11.41 | -11.36 | -9.67 | -0.36 | -0.52 | -3.90 | -2.88 | 0.79 | 0.53 |
| CH | -21.93 | -16.36 | -27.94 | -22.42 | -10.84 | -9.57 | -4.81 | -4.11 | -2.46 | -2.11 | -1.39 | -1.18 |
| $CH_2$ ($^3B_1$) | -17.79 | -12.58 | -22.86 | -17.89 | -7.80 | -7.12 | -2.82 | -2.34 | -1.16 | -1.00 | -0.53 | -0.43 |
| $CH_3$ | -18.66 | -16.48 | -20.14 | -15.48 | -7.00 | -6.77 | -2.32 | -1.83 | -0.95 | -0.85 | -0.43 | -0.33 |
| CN | -16.77 | -11.10 | -22.28 | -18.08 | -12.63 | -12.33 | -5.50 | -4.38 | -4.07 | -3.89 | -2.67 | -2.34 |
| F | -7.88 | -4.75 | -11.21 | -10.68 | -2.36 | -3.97 | -0.32 | -0.72 | -0.15 | -0.31 | -0.04 | -0.09 |
| HCO | -6.21 | -2.10 | -13.79 | -11.08 | -10.29 | -9.59 | -1.02 | -0.36 | -2.79 | -2.45 | 0.28 | 0.43 |
| $HO_2$ | -7.59 | -3.14 | -15.80 | -12.24 | -8.71 | -8.12 | -2.32 | -1.36 | -1.91 | -1.64 | -0.65 | -0.38 |
| N | -17.10 | -12.33 | -21.20 | -16.73 | -5.35 | -5.21 | -1.46 | -1.49 | -0.43 | -0.48 | -0.13 | -0.16 |
| NH | -15.73 | -10.51 | -20.91 | -16.26 | -6.81 | -6.30 | -2.35 | -1.91 | -1.00 | -0.82 | -0.48 | -0.35 |
| $NH_2$ | -11.42 | -6.76 | -18.06 | -13.82 | -6.16 | -6.14 | -1.92 | -1.48 | -0.80 | -0.71 | -0.36 | -0.26 |
| NO | -4.93 | -1.46 | -13.57 | -10.93 | -9.33 | -9.04 | -1.13 | -0.39 | -2.21 | -2.07 | 0.07 | 0.28 |
| O | -13.01 | -9.06 | -17.04 | -14.27 | -4.03 | -4.74 | -1.02 | -1.26 | -0.32 | -0.45 | -0.12 | -0.17 |
| $O_2$ | -1.94 | 0.21 | -13.32 | -10.42 | -7.69 | -7.74 | -1.57 | -0.62 | -1.33 | -1.32 | -0.44 | -0.14 |
| OF | -12.24 | -5.81 | -16.99 | -13.19 | -11.30 | -9.64 | -2.76 | -1.67 | -3.71 | -2.87 | -0.75 | -0.37 |
| OH | -9.98 | -5.48 | -15.57 | -12.30 | -5.22 | -5.38 | -1.42 | -1.11 | -0.66 | -0.58 | -0.27 | -0.19 |
| $\Delta$ | -12.84 | -8.30 | -18.60 | -14.84 | -8.22 | -7.78 | -2.31 | -1.78 | -1.80 | -1.58 | -0.55 | -0.40 |
| $\Delta_{std}$ | 6.14 | 5.50 | 5.10 | 3.81 | 2.87 | 2.25 | 1.52 | 1.23 | 1.27 | 1.05 | 0.81 | 0.69 |

Table S3: Recoveries of CCSDT/CCSD correlation energy differences in percent (%) for an ROHF reference.

| Molecule | CCSD(T) | | CCSD(T–2) | | CCSD(T–3) | | CCSD(T–4) | | CCSD(T–5) | | CCSD(T–6) | |
|---|---|---|---|---|---|---|---|---|---|---|---|---|
| | VDZ | VTZ | VDZ | VTZ | VDZ | VTZ | VDZ | VTZ | VDZ | VTZ | VDZ | VTZ |
| C | -24.37 | -17.78 | -32.12 | -25.01 | -13.95 | -10.94 | -8.02 | -6.00 | -5.87 | -4.23 | -5.03 | -3.52 |
| CCH | -6.60 | -2.77 | -17.23 | -13.23 | -8.17 | -8.63 | -1.52 | -0.78 | -0.61 | -0.97 | 0.37 | 0.35 |
| CF | -8.25 | -3.92 | -12.58 | -11.28 | -11.28 | -9.60 | -0.17 | -0.36 | -3.80 | -2.79 | 0.99 | 0.70 |
| CH | -21.49 | -15.78 | -29.08 | -23.13 | -12.27 | -10.44 | -6.33 | -5.02 | -4.00 | -3.05 | -2.95 | -2.12 |
| $CH_2$ ($^3B_1$) | -17.43 | -12.11 | -23.12 | -17.96 | -8.09 | -7.21 | -3.10 | -2.40 | -1.43 | -1.05 | -0.78 | -0.48 |
| $CH_3$ | -13.48 | -8.85 | -20.21 | -15.51 | -7.06 | -6.79 | -2.37 | -1.83 | -0.98 | -0.85 | -0.45 | -0.32 |
| CN | -6.95 | -2.82 | -15.45 | -12.38 | -10.17 | -10.40 | -1.22 | -0.38 | -2.05 | -2.27 | 0.44 | 0.61 |
| F | -7.89 | -4.58 | -12.43 | -10.93 | -3.66 | -4.23 | -1.62 | -0.97 | -1.44 | -0.55 | -1.32 | -0.33 |
| HCO | -5.46 | -1.52 | -14.35 | -11.26 | -11.12 | -9.96 | -1.73 | -0.59 | -3.69 | -2.87 | -0.44 | 0.20 |
| $HO_2$ | -7.37 | -2.91 | -16.27 | -12.33 | -9.24 | -8.23 | -2.81 | -1.41 | -2.43 | -1.71 | -1.12 | -0.40 |
| N | -17.25 | -12.35 | -20.91 | -17.79 | -4.99 | -6.35 | -1.08 | -2.67 | -0.05 | -1.66 | 0.25 | -1.34 |
| NH | -15.60 | -10.06 | -21.98 | -16.76 | -8.08 | -6.87 | -3.64 | -2.46 | -2.29 | -1.36 | -1.76 | -0.89 |
| $NH_2$ | -11.19 | -6.45 | -18.25 | -13.80 | -6.33 | -6.11 | -2.06 | -1.41 | -0.91 | -0.64 | -0.46 | -0.17 |
| NO | -3.12 | -0.12 | -14.41 | -11.22 | -10.79 | -9.79 | -2.39 | -0.92 | -3.79 | -2.91 | -1.27 | -0.32 |
| O | -13.15 | -8.79 | -18.68 | -15.02 | -5.87 | -5.54 | -2.88 | -2.06 | -2.18 | -1.25 | -1.97 | -0.96 |
| $O_2$ | -0.96 | 1.54 | -19.98 | -13.68 | -15.00 | -11.43 | -9.45 | -4.60 | -9.28 | -5.40 | -8.45 | -4.23 |
| OF | -11.44 | -5.24 | -16.50 | -12.77 | -11.11 | -9.41 | -2.26 | -1.21 | -3.45 | -2.60 | -0.24 | 0.10 |
| OH | -9.89 | -5.26 | -16.06 | -12.36 | -5.72 | -5.44 | -1.90 | -1.15 | -1.12 | -0.61 | -0.72 | -0.20 |
| $\Delta$ | -11.22 | -6.65 | -18.87 | -14.80 | -9.05 | -8.19 | -3.03 | -2.01 | -2.74 | -2.04 | -1.38 | -0.74 |
| $\Delta_{std}$ | 6.24 | 5.35 | 5.26 | 4.03 | 3.15 | 2.17 | 2.45 | 1.64 | 2.21 | 1.34 | 2.25 | 1.33 |

Table S4: Deviations from CCSDT correlation energies (in kcal/mol) for an RHF reference.

| Molecule | CCSD(T) | | CCSD(T–2) | | CCSD(T–3) | | CCSD(T–4) | | CCSD(T–5) | | CCSD(T–6) | |
|---|---|---|---|---|---|---|---|---|---|---|---|---|
| | VDZ | VTZ | VDZ | VTZ | VDZ | VTZ | VDZ | VTZ | VDZ | VTZ | VDZ | VTZ |
| $C_2H_2$ | 0.25 | 0.03 | 1.08 | 1.18 | 0.55 | 0.85 | 0.09 | 0.05 | 0.07 | 0.12 | 0.02 | 0.00 |
| $C_2H_4$ | 0.39 | 0.26 | 1.08 | 1.23 | 0.48 | 0.74 | 0.13 | 0.12 | 0.07 | 0.10 | 0.03 | 0.02 |
| $CH_2$ ($^1A_1$) | 0.45 | 0.51 | 0.62 | 0.77 | 0.28 | 0.39 | 0.16 | 0.20 | 0.10 | 0.13 | 0.08 | 0.10 |
| $CH_2O$ | 0.29 | 0.11 | 0.88 | 1.12 | 0.54 | 0.85 | 0.07 | 0.05 | 0.11 | 0.17 | 0.00 | -0.02 |
| CO | 0.29 | 0.09 | 0.85 | 1.09 | 0.74 | 1.05 | 0.02 | -0.02 | 0.20 | 0.27 | -0.05 | -0.08 |
| $CO_2$ | 0.15 | -0.13 | 1.27 | 1.67 | 1.36 | 1.82 | -0.09 | -0.17 | 0.42 | 0.54 | -0.15 | -0.22 |
| $F_2$ | 0.17 | -0.01 | 0.88 | 1.28 | 0.44 | 0.83 | 0.12 | 0.12 | 0.09 | 0.15 | 0.03 | 0.03 |
| $H_2O$ | 0.10 | 0.05 | 0.25 | 0.45 | 0.10 | 0.26 | 0.02 | 0.02 | 0.01 | 0.02 | 0.00 | 0.00 |
| $H_2O_2$ | 0.17 | -0.02 | 0.81 | 1.19 | 0.39 | 0.77 | 0.09 | 0.08 | 0.06 | 0.11 | 0.02 | 0.02 |
| HCN | 0.13 | -0.10 | 1.02 | 1.16 | 0.58 | 0.92 | 0.08 | 0.02 | 0.08 | 0.15 | 0.01 | -0.01 |
| HF | 0.06 | 0.02 | 0.12 | 0.32 | 0.05 | 0.19 | 0.00 | 0.01 | 0.01 | 0.02 | 0.00 | 0.00 |
| HNO | 0.20 | -0.02 | 1.09 | 1.38 | 0.65 | 1.05 | 0.14 | 0.12 | 0.15 | 0.23 | 0.05 | 0.03 |
| HOF | 0.18 | 0.02 | 0.80 | 1.20 | 0.42 | 0.82 | 0.09 | 0.08 | 0.08 | 0.15 | 0.02 | 0.01 |
| $N_2$ | 0.05 | -0.18 | 0.94 | 1.11 | 0.55 | 0.90 | 0.07 | 0.01 | 0.08 | 0.14 | 0.01 | -0.01 |
| $N_2H_2$ | 0.18 | -0.02 | 1.09 | 1.32 | 0.56 | 0.92 | 0.12 | 0.10 | 0.09 | 0.15 | 0.03 | 0.02 |
| $NH_3$ | 0.17 | 0.13 | 0.37 | 0.53 | 0.13 | 0.28 | 0.03 | 0.04 | 0.01 | 0.02 | 0.00 | 0.00 |
| $O_3$ | 0.08 | -0.44 | 3.69 | 4.10 | 3.32 | 4.06 | 0.42 | 0.11 | 1.33 | 1.67 | -0.08 | -0.34 |
| $\delta$ | 0.19 | 0.02 | 0.99 | 1.24 | 0.66 | 0.98 | 0.09 | 0.06 | 0.17 | 0.24 | 0.00 | -0.03 |
| $\delta_{std}$ | 0.11 | 0.20 | 0.76 | 0.82 | 0.75 | 0.88 | 0.10 | 0.08 | 0.31 | 0.39 | 0.05 | 0.10 |

Table S5: Deviations from CCSDT correlation energies (in kcal/mol) for a UHF reference.

| Molecule | CCSD(T) | | CCSD(T–2) | | CCSD(T–3) | | CCSD(T–4) | | CCSD(T–5) | | CCSD(T–6) | |
|---|---|---|---|---|---|---|---|---|---|---|---|---|
| | VDZ | VTZ | VDZ | VTZ | VDZ | VTZ | VDZ | VTZ | VDZ | VTZ | VDZ | VTZ |
| C | 0.20 | 0.29 | 0.23 | 0.36 | 0.08 | 0.13 | 0.03 | 0.05 | 0.01 | 0.02 | 0.01 | 0.01 |
| CCH | 1.01 | 0.90 | 1.60 | 1.74 | 0.79 | 1.06 | 0.33 | 0.34 | 0.22 | 0.27 | 0.14 | 0.15 |
| CF | 0.42 | 0.36 | 0.62 | 0.97 | 0.55 | 0.82 | 0.02 | 0.04 | 0.19 | 0.24 | -0.04 | -0.05 |
| CH | 0.32 | 0.40 | 0.41 | 0.55 | 0.16 | 0.24 | 0.07 | 0.10 | 0.04 | 0.05 | 0.02 | 0.03 |
| $CH_2$ ($^3B_1$) | 0.23 | 0.31 | 0.30 | 0.43 | 0.10 | 0.17 | 0.04 | 0.06 | 0.02 | 0.02 | 0.01 | 0.01 |
| $CH_3$ | 0.39 | 0.57 | 0.42 | 0.54 | 0.15 | 0.23 | 0.05 | 0.06 | 0.02 | 0.03 | 0.01 | 0.01 |
| CN | 1.55 | 1.44 | 2.07 | 2.34 | 1.17 | 1.60 | 0.51 | 0.57 | 0.38 | 0.50 | 0.25 | 0.30 |
| F | 0.05 | 0.11 | 0.07 | 0.25 | 0.01 | 0.09 | 0.00 | 0.02 | 0.00 | 0.01 | 0.00 | 0.00 |
| HCO | 0.43 | 0.23 | 0.96 | 1.20 | 0.71 | 1.04 | 0.07 | 0.04 | 0.19 | 0.27 | -0.02 | -0.05 |
| $HO_2$ | 0.44 | 0.35 | 0.92 | 1.35 | 0.51 | 0.90 | 0.14 | 0.15 | 0.11 | 0.18 | 0.04 | 0.04 |
| N | 0.08 | 0.20 | 0.10 | 0.27 | 0.03 | 0.08 | 0.01 | 0.02 | 0.00 | 0.01 | 0.00 | 0.00 |
| NH | 0.18 | 0.28 | 0.24 | 0.43 | 0.08 | 0.17 | 0.03 | 0.05 | 0.01 | 0.02 | 0.01 | 0.01 |
| $NH_2$ | 0.21 | 0.26 | 0.33 | 0.52 | 0.11 | 0.23 | 0.04 | 0.06 | 0.01 | 0.03 | 0.01 | 0.01 |
| NO | 0.36 | 0.17 | 0.99 | 1.28 | 0.68 | 1.06 | 0.08 | 0.05 | 0.16 | 0.24 | -0.01 | -0.03 |
| O | 0.07 | 0.18 | 0.09 | 0.29 | 0.02 | 0.10 | 0.01 | 0.03 | 0.00 | 0.01 | 0.00 | 0.00 |
| $O_2$ | 0.12 | -0.02 | 0.82 | 1.16 | 0.48 | 0.86 | 0.10 | 0.07 | 0.08 | 0.15 | 0.03 | 0.02 |
| OF | 0.70 | 0.62 | 0.97 | 1.41 | 0.65 | 1.03 | 0.16 | 0.18 | 0.21 | 0.31 | 0.04 | 0.04 |
| OH | 0.12 | 0.18 | 0.19 | 0.41 | 0.06 | 0.18 | 0.02 | 0.04 | 0.01 | 0.02 | 0.00 | 0.01 |
| $\delta$ | 0.38 | 0.38 | 0.63 | 0.86 | 0.35 | 0.56 | 0.09 | 0.11 | 0.09 | 0.13 | 0.03 | 0.03 |
| $\delta_{std}$ | 0.38 | 0.34 | 0.55 | 0.60 | 0.35 | 0.48 | 0.13 | 0.14 | 0.11 | 0.14 | 0.07 | 0.08 |

Table S6: Deviations from CCSDT correlation energies (in kcal/mol) for an ROHF reference.

| Molecule | CCSD(T) | | CCSD(T–2) | | CCSD(T–3) | | CCSD(T–4) | | CCSD(T–5) | | CCSD(T–6) | |
|---|---|---|---|---|---|---|---|---|---|---|---|---|
| | VDZ | VTZ | VDZ | VTZ | VDZ | VTZ | VDZ | VTZ | VDZ | VTZ | VDZ | VTZ |
| C | 0.20 | 0.29 | 0.26 | 0.41 | 0.11 | 0.18 | 0.06 | 0.10 | 0.05 | 0.07 | 0.04 | 0.06 |
| CCH | 0.47 | 0.28 | 1.24 | 1.34 | 0.59 | 0.87 | 0.11 | 0.08 | 0.04 | 0.10 | -0.03 | -0.04 |
| CF | 0.40 | 0.34 | 0.61 | 0.97 | 0.55 | 0.82 | 0.01 | 0.03 | 0.19 | 0.24 | -0.05 | -0.06 |
| CH | 0.32 | 0.40 | 0.43 | 0.58 | 0.18 | 0.26 | 0.09 | 0.13 | 0.06 | 0.08 | 0.04 | 0.05 |
| $CH_2$ ($^3B_1$) | 0.23 | 0.30 | 0.31 | 0.44 | 0.11 | 0.18 | 0.04 | 0.06 | 0.02 | 0.03 | 0.01 | 0.01 |
| $CH_3$ | 0.28 | 0.31 | 0.42 | 0.54 | 0.15 | 0.24 | 0.05 | 0.06 | 0.02 | 0.03 | 0.01 | 0.01 |
| CN | 0.64 | 0.36 | 1.43 | 1.58 | 0.94 | 1.33 | 0.11 | 0.05 | 0.19 | 0.29 | -0.04 | -0.08 |
| F | 0.05 | 0.11 | 0.08 | 0.26 | 0.02 | 0.10 | 0.01 | 0.02 | 0.01 | 0.01 | 0.01 | 0.01 |
| HCO | 0.39 | 0.17 | 1.01 | 1.24 | 0.79 | 1.09 | 0.12 | 0.07 | 0.26 | 0.32 | 0.03 | -0.02 |
| $HO_2$ | 0.44 | 0.32 | 0.96 | 1.37 | 0.55 | 0.92 | 0.17 | 0.16 | 0.14 | 0.19 | 0.07 | 0.04 |
| N | 0.08 | 0.20 | 0.10 | 0.29 | 0.02 | 0.11 | 0.01 | 0.04 | 0.00 | 0.03 | 0.00 | 0.02 |
| NH | 0.18 | 0.27 | 0.26 | 0.46 | 0.09 | 0.19 | 0.04 | 0.07 | 0.03 | 0.04 | 0.02 | 0.02 |
| $NH_2$ | 0.21 | 0.25 | 0.34 | 0.53 | 0.12 | 0.23 | 0.04 | 0.05 | 0.02 | 0.02 | 0.01 | 0.01 |
| NO | 0.23 | 0.01 | 1.08 | 1.34 | 0.81 | 1.17 | 0.18 | 0.11 | 0.28 | 0.35 | 0.09 | 0.04 |
| O | 0.07 | 0.18 | 0.10 | 0.31 | 0.03 | 0.11 | 0.02 | 0.04 | 0.01 | 0.03 | 0.01 | 0.02 |
| $O_2$ | 0.07 | -0.18 | 1.36 | 1.62 | 1.02 | 1.36 | 0.64 | 0.55 | 0.63 | 0.64 | 0.58 | 0.50 |
| OF | 0.66 | 0.57 | 0.96 | 1.38 | 0.64 | 1.02 | 0.13 | 0.13 | 0.20 | 0.28 | 0.01 | -0.01 |
| OH | 0.12 | 0.18 | 0.20 | 0.42 | 0.07 | 0.19 | 0.02 | 0.04 | 0.01 | 0.02 | 0.01 | 0.01 |
| $\delta$ | 0.28 | 0.24 | 0.62 | 0.84 | 0.38 | 0.58 | 0.10 | 0.10 | 0.12 | 0.15 | 0.05 | 0.03 |
| $\delta_{std}$ | 0.19 | 0.16 | 0.47 | 0.50 | 0.35 | 0.48 | 0.15 | 0.12 | 0.16 | 0.17 | 0.14 | 0.12 |

Table S7: CCSDT and CCSD(T) recoveries of CCSDTQ correlation energies in percent (%) for RHF, UHF, and ROHF references.

| Molecule | RHF | | | | Molecule | UHF | | | | ROHF | | | |
|---|---|---|---|---|---|---|---|---|---|---|---|---|---|
| | CCSDT | | CCSD(T) | | | CCSDT | | CCSD(T) | | CCSDT | | CCSD(T) | |
| | VDZ | VTZ | VDZ | VTZ | | VDZ | VTZ | VDZ | VTZ | VDZ | VTZ | VDZ | VTZ |
| $C_2H_2$ | -7.36 | -6.31 | -10.55 | -6.61 | C | -2.30 | -1.62 | -26.86 | -19.85 | -0.55 | -0.49 | -24.78 | -18.18 |
| $C_2H_4$ | -5.29 | -4.43 | -11.03 | -6.99 | CCH | -7.51 | -6.53 | -20.55 | -14.81 | -7.50 | -6.64 | -13.60 | -9.23 |
| $CH_2$ ($^1A_1$) | -4.81 | -3.79 | -23.75 | -17.68 | CF | -6.34 | -3.19 | -14.42 | -7.32 | -6.32 | -3.20 | -14.05 | -7.00 |
| $CH_2O$ | -8.03 | -5.03 | -12.17 | -5.99 | CH | -3.14 | -2.24 | -24.38 | -18.24 | -3.10 | -2.25 | -23.92 | -17.68 |
| CO | -7.88 | -5.39 | -11.66 | -6.14 | $CH_2$ ($^3B_1$) | -3.72 | -1.96 | -20.85 | -14.30 | -3.74 | -2.00 | -20.52 | -13.87 |
| $CO_2$ | -8.79 | -5.56 | -10.01 | -4.87 | $CH_3$ | -1.72 | -0.67 | -20.06 | -17.05 | -3.50 | -2.25 | -16.50 | -10.91 |
| $F_2$ | -14.21 | -7.16 | -16.70 | -7.12 | CN | -8.68 | -7.33 | -23.99 | -17.62 | -8.55 | -7.41 | -14.91 | -10.01 |
| $H_2O$ | -12.44 | -3.97 | -16.88 | -4.92 | F | -10.74 | -1.56 | -17.78 | -6.23 | -10.56 | -1.56 | -17.62 | -6.06 |
| $H_2O_2$ | -12.04 | -5.86 | -14.65 | -5.72 | HCO | -7.76 | -5.16 | -13.49 | -7.15 | -7.72 | -5.17 | -12.76 | -6.61 |
| HCN | -9.25 | -7.27 | -10.76 | -6.47 | $HO_2$[a] | -10.67 | | -17.45 | | -10.60 | | -17.19 | |
| HF | -16.35 | -3.17 | -20.07 | -3.62 | N | -5.21 | -1.57 | -21.42 | -13.71 | -5.22 | -1.59 | -21.57 | -13.74 |
| HNO | -10.75 | -7.11 | -13.04 | -6.96 | NH | -6.46 | -2.35 | -21.17 | -12.61 | -6.38 | -2.41 | -20.99 | -12.23 |
| HOF | -12.46 | -5.99 | -15.21 | -6.13 | $NH_2$ | -7.04 | -3.12 | -17.66 | -9.67 | -6.99 | -3.13 | -17.40 | -9.38 |
| $N_2$ | -10.87 | -7.90 | -11.44 | -6.48 | NO | -9.77 | -6.38 | -14.21 | -7.74 | -9.77 | -6.49 | -12.59 | -6.60 |
| $N_2H_2$ | -8.82 | -6.33 | -11.03 | -6.15 | O | -8.30 | -1.54 | -20.24 | -10.45 | -8.07 | -1.54 | -20.16 | -10.19 |
| $NH_3$ | -7.24 | -3.54 | -13.39 | -6.14 | $O_2$ | -14.93 | -8.39 | -16.58 | -8.20 | -14.60 | -8.67 | -15.42 | -7.27 |
| $O_3$ | -13.93 | -10.73 | -14.27 | -9.36 | OF | -9.73 | -4.67 | -20.78 | -10.21 | -9.71 | -4.68 | -20.05 | -9.68 |
| | | | | | OH | -11.86 | -2.98 | -20.66 | -8.29 | -11.73 | -2.98 | -20.46 | -8.08 |
| $\Delta$ | -10.03 | -5.85 | -13.92 | -6.90 | $\Delta$ | -7.55 | -3.60 | -19.59 | -11.97 | -7.48 | -3.67 | -18.03 | -10.40 |
| $\Delta_{std}$ | 3.23 | 1.89 | 3.72 | 3.02 | $\Delta_{std}$ | 3.50 | 2.35 | 3.60 | 4.40 | 3.47 | 2.40 | 3.72 | 3.69 |

[a] Due to convergence issues for the CCSDTQ calculation, no cc-pVTZ results are presented here for $HO_2$.

Table S8: CCSDT and CCSD(T) deviations from CCSDTQ correlation energies (in kcal/mol) for RHF, UHF, and ROHF references.

| Molecule | RHF | | | | Molecule | UHF | | | | ROHF | | | |
|---|---|---|---|---|---|---|---|---|---|---|---|---|---|
| | CCSDT | | CCSD(T) | | | CCSDT | | CCSD(T) | | CCSDT | | CCSD(T) | |
| | VDZ | VTZ | VDZ | VTZ | | VDZ | VTZ | VDZ | VTZ | VDZ | VTZ | VDZ | VTZ |
| $C_2H_2$ | 0.57 | 0.69 | 0.82 | 0.73 | C | 0.02 | 0.03 | 0.21 | 0.32 | 0.00 | 0.01 | 0.20 | 0.30 |
| $C_2H_4$ | 0.36 | 0.45 | 0.76 | 0.71 | CCH | 0.58 | 0.71 | 1.60 | 1.60 | 0.58 | 0.72 | 1.06 | 1.00 |
| $CH_2$ ($^1A_1$) | 0.11 | 0.14 | 0.57 | 0.65 | CF | 0.33 | 0.28 | 0.75 | 0.64 | 0.33 | 0.28 | 0.73 | 0.62 |
| $CH_2O$ | 0.57 | 0.55 | 0.86 | 0.66 | CH | 0.05 | 0.06 | 0.37 | 0.46 | 0.05 | 0.06 | 0.37 | 0.45 |
| CO | 0.60 | 0.61 | 0.88 | 0.70 | $CH_2$ ($^3B_1$) | 0.05 | 0.05 | 0.28 | 0.35 | 0.05 | 0.05 | 0.28 | 0.35 |
| $CO_2$ | 1.10 | 1.04 | 1.25 | 0.91 | $CH_3$ | 0.04 | 0.02 | 0.42 | 0.59 | 0.08 | 0.08 | 0.36 | 0.39 |
| $F_2$ | 0.96 | 0.87 | 1.13 | 0.86 | CN | 0.88 | 1.03 | 2.44 | 2.46 | 0.86 | 1.02 | 1.51 | 1.38 |
| $H_2O$ | 0.29 | 0.20 | 0.39 | 0.25 | F | 0.07 | 0.04 | 0.12 | 0.15 | 0.07 | 0.04 | 0.12 | 0.15 |
| $H_2O_2$ | 0.80 | 0.71 | 0.98 | 0.70 | HCO | 0.58 | 0.59 | 1.01 | 0.82 | 0.59 | 0.60 | 0.98 | 0.77 |
| HCN | 0.77 | 0.87 | 0.90 | 0.78 | $HO_2$[a] | 0.70 | | 1.14 | | 0.70 | | 1.14 | |
| HF | 0.25 | 0.13 | 0.30 | 0.15 | N | 0.03 | 0.03 | 0.11 | 0.23 | 0.03 | 0.03 | 0.11 | 0.23 |
| HNO | 0.92 | 0.95 | 1.12 | 0.93 | NH | 0.08 | 0.06 | 0.25 | 0.34 | 0.08 | 0.07 | 0.26 | 0.34 |
| HOF | 0.82 | 0.72 | 1.00 | 0.74 | $NH_2$ | 0.14 | 0.12 | 0.35 | 0.38 | 0.14 | 0.12 | 0.35 | 0.37 |
| $N_2$ | 0.91 | 0.98 | 0.96 | 0.80 | NO | 0.79 | 0.80 | 1.15 | 0.97 | 0.81 | 0.83 | 1.04 | 0.84 |
| $N_2H_2$ | 0.73 | 0.80 | 0.91 | 0.78 | O | 0.05 | 0.03 | 0.12 | 0.21 | 0.05 | 0.03 | 0.12 | 0.21 |
| $NH_3$ | 0.20 | 0.18 | 0.37 | 0.31 | $O_2$ | 1.09 | 1.02 | 1.21 | 0.99 | 1.16 | 1.13 | 1.23 | 0.94 |
| $O_3$ | 3.32 | 3.45 | 3.40 | 3.01 | OF | 0.62 | 0.53 | 1.32 | 1.15 | 0.62 | 0.53 | 1.29 | 1.10 |
| | | | | | OH | 0.16 | 0.10 | 0.28 | 0.29 | 0.16 | 0.10 | 0.28 | 0.28 |
| $\delta$ | 0.78 | 0.79 | 0.98 | 0.80 | $\delta$ | 0.35 | 0.32 | 0.73 | 0.70 | 0.35 | 0.33 | 0.63 | 0.57 |
| $\delta_{std}$ | 0.72 | 0.75 | 0.68 | 0.61 | $\delta_{std}$ | 0.35 | 0.37 | 0.64 | 0.60 | 0.36 | 0.38 | 0.48 | 0.37 |

[a] Due to convergence issues for the CCSDTQ calculation, no cc-pVTZ results are presented here for $HO_2$.
